# Supplementary material for: Automated Recurrence Analysis for Almost-Linear Expected-Runtime Bounds
Source: arXiv:1705.00314 source file (2017-04-30)
Supplement: Supplementary file 1 [file for_appendix.tex]

%%% RANOMDIZED SEARCH

\lstset{language=prog}
\lstset{tabsize=3}
\newsavebox{\progsearch}
\begin{lrbox}{\progsearch}
\begin{lstlisting}[mathescape]
$\mathsf{randsearch}(ar,i,j,d)$ {
1:  if ($i=j$ and $ar[i]\ne d$)
2:   return $-1$;
3:  else if ($i=j$ and $ar[i]=d$)
4:   return $i$;
5:  else
6:   $k\leftarrow \mathrm{uniform}(i,j)$;

7:   if ($ar[k]=d$)
8:    return $k$;
9:   else if ($ar[k]<d$ and $k<j$)
10:   return $\mathsf{randsearch}(ar, k+1, j,d)$;
11:  else if ($ar[k]>d$ and $i<k$)
12:   return $\mathsf{randsearch}(ar,1,k-1,d)$;
13:  else
14:   return $-1$;
     end if
    end if
}
\end{lstlisting}
\end{lrbox}

\begin{figure}
%%[11]{r}{5.5cm}
\usebox{\progsearch}
\caption{Sherwood's {\sc Randomized-Search}}
\label{fig:randsearch}
\end{figure}

The description of the pseudo-code is as follows.
The first four lines deal with the base case when there is only one index in the index range.
The remaining lines deal with the recursive case:
in line 6, an index $k$ is uniformly sampled from $\{i,i+1,\dots,j\}$;
line 7--8 check whether $k$ is the output;
line 9--12 perform the recursive calls depending on whether $ar[k]<d$ or not;
finally, line 13--14 handle the case when $d<ar[i]$ or $d>ar[j]$.

%%%%%%% QUICKSORT

\lstset{language=prog}
\lstset{tabsize=3}
\newsavebox{\progsort}
\begin{lrbox}{\progsort}
\begin{lstlisting}[mathescape]
$\mathsf{quicksort}(ar,i,j)$ {
1: if ($i<j$)
2:   $k\leftarrow \mathrm{uniform}(i,j)$;
3:   $m\leftarrow \mathsf{pivot}(ar,i,j,ar[k])$;

4:   if ($i\le m-1$)
5:     $\mathsf{quicksort}(ar,i,m-1)$;
     end if

6:   if ($m+1\le j$)
7:     $\mathsf{quicksort}(ar,m+1,j)$;
     end if
   end if
}
\end{lstlisting}
\end{lrbox}

\begin{figure}
\centering
\usebox{\progsort}
\caption{Randomized {\sc Quick-Sort}}
\label{fig:quicksort}
\end{figure}

depicted in Fig.~\ref{fig:quicksort}, where every input $(ar,i,j)$ is assumed to satisfy that $0\le i\le j$ and $ar$ is an array of integers which does not contain duplicate numbers.

The description of the pseudo-code is as follows:
first, line 2 samples an integer uniformly from $\{i,\dots, j\}$;
then, line 3 calls a subroutine $\mathsf{pivot}$ which (i) rearranges $ar$ such that integers in $ar$ which are less than $ar[k]$ come first,
then $ar[k]$, and finally integers in $ar$ greater than $ar[k]$, and (ii) outputs the new index $m$ of $ar[k]$ in $ar$; and
finally, lines 4--7 handle recursive calls to sub-arrays.

From the pseudo-code, the following recurrence relation is easily obtained:

 %%%%%%%%%%%% QUICK SELECT

 depicted in Fig.~\ref{fig:quickselect} which upon any input $(ar,i,j)$ and $d$ such that
$0\le i\le j$, $1\le d\le j-i+1$ and $ar$ contains no duplicate integers, finds the $d$-th largest integer in $ar$.
Note that for an array of size $n$, and $d=n/2$, we have the {\sc Median-Find} algorithm.

The description of the pseudo-code is as follows: line 1 handles the base case;
line 3 starts the recursive case by sampling $k$ uniformly from $\{i,\dots,j\}$;
line 4 rearranges $ar$ and returns an $m$ in the same way as $\mathsf{pivot}$ in {\sc Quick-Sort}
(cf. Example~\ref{ex:quicksort});
line 5 handles the case when $ar[k]$ happens to be the $d$-th largest integer in $ar$;
and finally, line 7--10 handle the recursive calls.

The recurrence relation for this example is

\lstset{language=prog}
\lstset{tabsize=3}
\newsavebox{\progdiameter}
\begin{lrbox}{\progdiameter}
\begin{lstlisting}[mathescape]
$\mathsf{diameter}(S)$ {
1: if ($|S|=1$)
2:  return 0;
   else
3:  $p\leftarrow \mathrm{uniform}(S)$;
4:  $d\leftarrow \max_{p'\in S} \mbox{\sl dist}(p,p')$
5:  $U\leftarrow \bigcap_{p'\in S}\{p''\in\Rset^3 \mid  \mbox{\sl dist}(p'',p')\le d\}$
6:  $S'\leftarrow S\backslash U$

7:  if ($S'=\emptyset$)
8:   return $d$
9:   else
10:   return $\mathsf{diameter}(S')$
     end if
    end if
}
\end{lstlisting}
\end{lrbox}

\lstset{language=prog}
\lstset{tabsize=3}
\newsavebox{\progselect}
\begin{lrbox}{\progselect}
\begin{lstlisting}[mathescape]
$\mathsf{quickselect}(ar,i,j,d)$ {
1: if ($i=j$) return $a[i]$;
2: else
3:  $k\leftarrow \mathrm{uniform}(i,j)$;
4:  $m\leftarrow \mathsf{pivot}(ar,i,j,ar[k])$;

5:  if ($m-i+1=d$)
6:   return $ar[m]$;
7:  else if ($m-i+1<d$)
8:   return $\mathsf{quickselect}(ar,m+1,j,d)$;
9:  else if ($m-i+1>d$)
10:  return $\mathsf{quickselect}(ar,i,m-1,d)$;
    end if
   end if
}
\end{lstlisting}
\end{lrbox}
\begin{figure}
\begin{minipage}{0.55\textwidth}
\centering
\usebox{\progselect}
\caption{Randomized {\sc Quick-Select}}
\label{fig:quickselect}
\end{minipage}
\begin{minipage}{0.45\textwidth}
\centering
\usebox{\progdiameter}
\caption{{\sc Diameter-Computation}}
\label{fig:diameter}
\end{minipage}
\end{figure}

%%% DIAMETER

A pseudo-code to implement this is depicted in Fig.~\ref{fig:diameter}.

The description of the pseudo-code is as follows:
line 1--2 handle the base case;
line 3 samples a point $p$ uniformly from $S$;
line 4 calculates the maximum distance in $S$ from $p$;
line 5 calculates the intersection of all balls centered at points in $S$ with uniform radius $d$;
line 6 calculates the set of points outside $U$;
lines 7--8 handle the situation $S'=\emptyset$ which implies that $d$ is the diameter;
lines 9--10 handle the recursive call to $S'$.
Due to uniform choice of $p$ at line 3, the size of $S'$ is uniformly in $[0,|S|-1]$;
it then follows a pivoting (similar to that in Example~\ref{ex:quickselect} and Example~\ref{ex:quicksort}) by line $5$
w.r.t the linear order over $\{\max_{p'\in S}{\mbox{\sl dist}(p,p')}\mid p\in S\}$.

Lines 5--6 can be done in $\mathcal{O}(|S|\cdot \log{|S|})$ time for Euclidean distance,
and  $\mathcal{O}(|S|)$ time for $L_1$ metric~\cite{DBLP:books/cu/MotwaniR95}.

%%% SORT WITH QUICKSELECT

\lstset{language=prog}
\lstset{tabsize=3}
\newsavebox{\progsortselect}
\begin{lrbox}{\progsortselect}
\begin{lstlisting}[mathescape]

$\mathsf{sortbyselect}(ar,i,j)$ {
1:  if ($i<j$)
2:    $m\leftarrow \mathsf{quickselect}(ar,i,j,\lfloor\frac{j-i+1}{2}\rfloor)$;
3:    if ($i< m-1$)
4:      $\mathsf{sortbyselect}(ar,i,m-1)$;
      end if

5:    if ($m+1<j$)
6:      $\mathsf{sortbyselect}(ar,m+1,j)$;
      end if
    end if
}
\end{lstlisting}
\end{lrbox}
\begin{figure}
\centering
\usebox{\progsortselect}
\caption{Sorting with {\sc Quick-Select}}
\label{fig:sortselect}
\end{figure}

%%%%% OVERAPPROXIMATIONS

We have the following result using integral-by-part technique
and Newton-Leibniz Formula.

%\smallskip
\begin{lemma}\label{lemm:basiccalculus}
For all $a,b\in (0,\infty)$ such that $a<b$, the following assertions hold:
\begin{eqnarray*}
\displaystyle
(1)\ \int_a^b \frac{1}{x}\,\mathrm{d}x  =   \ln{x}{\Big|}_{a}^b \enspace ; \displaystyle
~~~(2)\  \int_a^b \ln{x}\,\mathrm{d}x  =  \left(x\cdot\ln{x}-x\right){\Big|}_{a}^b \enspace\\[1ex]
\displaystyle
(3)\ \int_a^b x\cdot\ln{x}\,\mathrm{d}x  =  \left(\frac{1}{2}\cdot x^2\cdot\ln{x}-\frac{1}{4}\cdot x^2\right){\Big|}_{a}^b~~ \enspace.
\end{eqnarray*}
\end{lemma}

In the following lemma we provide a tight approximation for floored expressions, the proof of which is a simple case distinction between
even and odd cases.

%\smallskip
\begin{lemma}\label{lemm:flooroverapprox}
For all natural numbers $n$, we have
$\frac{n-1}{2}\le \left\lfloor\frac{n}{2}\right\rfloor\le \frac{n}{2}\le \left\lceil\frac{n}{2}\right\rceil \le \frac{n+1}{2}$~~.
\end{lemma}

The following lemma handles over-approximation of simple summations.

%\smallskip
\begin{lemma}\label{lemm:sumoverapprox}
For any natural number $n\ge 2$ and real number $c$, one has that
$\frac{\sum_{j=1}^{n-1} c}{n}\le c\mbox{ and }\frac{\left( \sum_{j=\left\lceil\frac{\mathfrak{n}}{2}\right\rceil}^{n-1} c+ \sum_{j=\left\lfloor\frac{\mathfrak{n}}{2}\right\rfloor}^{n-1} c\right)}{n}\le c$~~.
\end{lemma}

Based on Lemma~\ref{lemm:flooroverapprox} and Taylor's Theorem, we have the following two propositions.

%%%Example OVERAPPROX

Consider the summation
\[
\displaystyle\sum_{j=\left\lceil\frac{n}{2}\right\rceil}^{n-1}\ln{j}+ \displaystyle\sum_{j=\left\lfloor\frac{n}{2}\right\rfloor}^{n-1} \ln{j}\quad (n\ge 4).
\]
By Proposition~\ref{prop:integralapproximation}, we can over-approximate it as
\[
2\cdot\left(\Gamma_{\ln{\mathfrak{n}}}\left(n\right)+\frac{1}{12}\right)
-\left(\Gamma_{\ln{\mathfrak{n}}}\left(\left\lceil\frac{n}{2}\right\rceil\right)+\Gamma_{\ln{\mathfrak{n}}}\left(\left\lfloor\frac{n}{2}\right\rfloor\right)-0.5402\right)
\]
which is equal to
\begin{align*}
& 2\cdot n\cdot\ln{n}-2\cdot n-\ln{n}-\left\lceil\frac{n}{2}\right\rceil\cdot\ln{\left\lceil\frac{n}{2}\right\rceil}-\left\lfloor\frac{n}{2}\right\rfloor\cdot\ln{\left\lfloor\frac{n}{2}\right\rfloor}\\
&{}+\left\lceil\frac{n}{2}\right\rceil+\left\lfloor\frac{n}{2}\right\rfloor+\frac{\ln{\left\lfloor\frac{n}{2}\right\rfloor}}{2}+\frac{\ln{\left\lceil\frac{n}{2}\right\rceil}}{2}+\frac{1}{6}+0.5402.
\end{align*}
Then using Proposition~\ref{prop:lnflooroverapprox}, we can further obtain the following over-approximation
\begin{align*}
& 2\cdot n\cdot\ln{n}-2\cdot n-\ln{n}+0.7069-\frac{n}{2}\cdot\left(\ln{n}-\ln{2}\right)-\frac{n-1}{2}\cdot\left(\ln{n}-\ln{2}-\frac{1}{n-1}\right)\\
&{}+\frac{n+1}{2}+\frac{n}{2}+\frac{\ln{n}-\ln{2}}{2}+\frac{\ln{n}-\ln{2}+\frac{1}{n}}{2}
\end{align*}
which is roughly
$n\cdot\ln{n}-(1-\ln{2})\cdot n+\frac{1}{2}\cdot\ln{n}+0.6672+\frac{1}{2\cdot n}$.

\vspace{-1em}
\subsection{Discussion}
\vspace{-0.5em}
We discuss some aspects of the recurrence relations we consider and possible generalizations.
\begin{compactenum}

\item {\em Recurrence relations.} 
We note that the recurrence relations we consider capture various classical randomized programs, 
ranging for sorting ({\sc Quick-Sort}), searching ({\sc Randomized-Search}), {\sc Resource-Allocation}, 
{\sc Coupon-Collector}, which are basic in several analysis.
Thus the recurrence relations we consider indeed captures a diverse range of widely used programs 
such as sort, search, etc.

\item {\em Generalization of recurrence relations.}
Our setting of recurrence relations can also be easily generalized.
For example, consider a restricted non-uniform sampling that has one uniform probability value for 
the first half of the array, and a different uniform value for the second half. 
Then we can truncate the summation (for expected-time complexity) into two halves and apply our methods.
%% with little changes.

\item {\em Generalization of bounds.}
In this work we focus on almost-linear bounds.
Our approach could be extended to upper bounds such as $\mathcal{O}\left(n^k\right)$ or 
$\mathcal{O}\left(n^k\cdot \log n\right)$ ($k\ge 2$) since the definite integral over these 
functions can be obtained in closed form through integral-by-part technique, and 
can be approximated efficiently as in Proposition~\ref{prop:integralapproximation}.

\end{compactenum}
While our techniques can be generalized to other recurrence relations and bounds, 
in this work we focus on the recurrence relations and bounds for two reasons:
(a)~most of the classical examples does not require such generalizations; and 
(b)~the simpler classes allow clear exposition of the core ideas.
